# Supplementary material for: Transition dynamics in aging systems: microscopic origin of logarithmic time evolution
Source: arXiv:1208.1383 source file (2013-03-26)
Supplement: Supplementary file 1 [file supplementary.pdf]

# Supplementary Material: Transition dynamics in aging systems: microscopic origin of logarithmic time evolution

Michael A. Lomholt,[1] Ludvig Lizana,[2,3] Ralf Metzler,[4,5] and Tobias Ambjörnsson[6]

[1]*MEMPHYS, Department of Physics, Chemistry and Pharmacy, University of Southern Denmark, DK-5230 Odense M, Denmark*
[2]*Department of Physics and Center for Soft Matter Research, New York University, 4 Washington Place, New York, NY 10003, USA*
[3]*Integrated Science Lab, Department of Physics, Umeå University, SE-901 87 Umeå, Sweden*
[4]*Institute for Physics and Astronomy, University of Potsdam, D-14476 Potsdam-Golm, Germany*
[5]*Department of Physics, Tampere University of Technology, FI-33101 Tampere, Finland*
[6]*Department of Astronomy and Theoretical Physics, Lund University, SE-22362 Lund, Sweden*

## Interpretation of Eq. (5) in the main text in terms of products of random variables

Let us introduce $\lambda(x) = G(x)/x$ (i.e. $\lambda(p) = G(p-1)$ in Mellin space), where the quantity $G(x)$ is defined in the main text. Eq. (5) in the text can then be written

$$\rho_n(t) = \int_0^\infty \rho_{n-1}(t')\lambda(t/t')t'^{-1}dt'. \tag{1}$$

Interestingly, this is the transform of the product of two random numbers [1]. Therefore, denoting by $\hat{t}_n$ the random arrival time at state $n$ the equation above states that $\hat{t}_n = \hat{\chi}_n \hat{t}_{n-1}$, where $\hat{\chi}_n$ is an independent random number taken from the distribution $\lambda(\chi)$. This means that we may write $\hat{t}_n = \hat{\chi}_n \hat{t}_{n-1} = \hat{\chi}_n \cdots \hat{\chi}_1 t_0$, or $\ln(\hat{t}_n/t_0) = \sum_{i=1}^n \ln \hat{\chi}_i$, i.e. the arrival time $t_n$ at state $n$ is a sum in logarithmic time. For the case $0 < \alpha < 1$ we find that at large $n$ the quantity $\hat{z}_i = \ln \hat{\chi}_i$ has distribution

$$\langle \delta(z - \hat{z}_i)\rangle = e^z \lambda(e^z) = \frac{\sin(\pi\alpha)}{\pi} \frac{\theta(z)}{(e^z - 1)^\alpha}, \tag{2}$$

with the moment generating function $G(p) = \langle e^{p\hat{z}_i}\rangle = \Gamma(\alpha - p)/[\Gamma(\alpha)\Gamma(1-p)]$ and cumulants $\kappa_m = (d/dp)^m \ln G(p)|_{p=0}$. From the central limit theorem we infer that $\ln(\hat{t}_n/t_0)$ is normally distributed with average $n\mu$ and variance $n\sigma^2$ which implies the Gaussian form for $n \to \infty$

$$\rho_n(t) \sim \frac{1}{t\sqrt{2\pi\sigma^2 n}} \exp\left(-\frac{(\ln(t/t_0) - n\mu)^2}{2n\sigma^2}\right) \tag{3}$$

The mapping above of our problem to that of a product of random numbers provide a simple explanation for the appearance of logarithmic time dependence of the quantities studied in the main text.

If we take the limit $t \to \infty$ (keeping $n$ finite) we find the asymptotic behaviour

$$\rho_n(t) \sim \frac{1}{(n-1)!}\left[\frac{\sin(\alpha\pi)}{\pi}\right]^n \left[\ln\left(\frac{t}{t_0}\right)\right]^{n-1} \frac{t_0^\alpha}{t^{1+\alpha}}. \tag{4}$$

Thus, the distribution of arrival times at state $n$ mirrors the power-law tail of the original distribution $\psi(\tau)$ plus a logarithmic correction with power $n$.

## Asymptotic expression for $\langle n^q(p)\rangle$

To find $\langle n^q(p)\rangle$ we note that $G(p)$ (see Eq. (6) in main text) is an increasing function of $p$ (as long as $p < \alpha$) which grows larger than unity for $p > 0$. The moments therefore diverge as $p \to 0^-$, and have the fundamental strip $-\infty < p < 0$. The long time asymptotic behavior of the moments is therefore dominated by the singularity at $p \sim 0$. Expanding $G(p)$ at $p \sim 0$ to second order, $G(p) \sim 1 + \mu p + \frac{1}{2}(\sigma^2 + \mu^2)p^2$. If we similarly expand the sum over $n$ in $\langle n^q(p)\rangle$ in deviations of $G(p)$ from unity, keeping the lowest and next to lowest order contributions, we find

$$\sum_{n=0}^\infty n^q G(p)^n \sim \frac{G(p)^q q!}{[1 - G(p)]^{q+1}} + \frac{(q-1)G(p)^{q-1}q!}{2[1-G(p)]^q}. \tag{5}$$

Collecting terms we finally obtain Eq. (7) in the main text.

## The full distribution, $h_n(t)$

To obtain the full form of the distribution $h_n(t)$ we note that its Mellin transform, Eq. (6) in the main text, can be rephrased as $h_n(p) = t_0^p e^{n\ln G(p)}[G(p) - 1]/p$. In the large $n$ limit, $h_n$ is different from zero only for $p \approx 0$. To obtain an approximate result for $h_n(t)$ we expand $h_n(p)$ for large $n$ and small $p$, keeping the product $np^\nu$ constant. The scaling exponent $\nu$ is chosen as small as possible while still obtaining a non-trivial result when discarding the small terms. For $\nu = 1$ a $\delta$-function is obtained for $h_n(t)$, for $\nu = 2$ we find to zeroth order in small quantities $h_n^{(0)}(p) = \mu t_0^p \exp[n(\mu p + \sigma^2 p^2/2)]$, thus

$$h_n^{(0)}(t) = \frac{\mu}{\sqrt{2\pi\sigma^2 n}} \exp\left(-\frac{(\ln(t/t_0) - \mu n)^2}{2\sigma^2 n}\right). \tag{6}$$

This expression systematically improves by inclusion of higher order terms in $p$ and $np^3$. To first order, $h_n^{(1)}(p) =$

$h_n^{(0)}(p)[1+(\sigma^2+\mu^2)p/(2\mu)+\kappa_3 np^3/6]$, thus

$$h_n^{(1)}(t) = h_n^{(0)}(t)\left[1+\frac{\sigma^2+\mu^2}{2\mu\sqrt{\sigma^2 n}}y+\frac{\kappa_3 n}{6(\sigma^2 n)^{3/2}}(y^3-3y)\right], \quad (7)$$

where $y = [\ln(t/t_0) - \mu n]/\sqrt{\sigma^2 n}$.

**Relation to a simple glass model**

The equations derived here apply more generally beyond the ageing waiting time process considered in the text. In fact, for Eq. (5) in the main text to hold it only requires that the distribution $\psi_1$ can be written in the form $\psi_1(t-t'|t') = t'^{-1}\lambda(t/t')\theta(t-t')$. This holds as long as there is no time scale in the problem other than the arrival time $t'$. Moreover, we require that $G(p)$ can be Taylor expanded. An example where these conditions are met is the random walk model for transitions between energy minima in a simple glass proposed by Angelani et al. [2]. They found that the rate of transitions decays as $c/t$, where $c > 0$ is a numerical constant. This corresponds to the waiting time distribution $\psi_1(t-t'|t') = ct'^c\theta(t-t')/t^{1+c}$ and moment generating function $G(p) = 1/(1-p/c)$. Our main equations therefore apply to this process with $\mu = 1/c$, $\sigma = 1/c^2$ and $\kappa_3 = 2/c^3$.

[1] A.G. Glen, L.M. Leemis, and J.H. Drew, Computational statistics & data analysis **44**, 451 (2004).

[2] L. Angelani, R. Di Leonardo, G. Parisi, and G. Ruocco, Phys. Rev. Lett. **87**, 055502 (2001).
